# Supplementary material for: Language Model Can Do Knowledge Tracing: Simple but Effective Method to Integrate Language Model and Knowledge Tracing Task
Source: arXiv:2406.02893 source file (2024-06-09)
Supplement: Supplementary file 1 [file 6_appendix.tex]

\newpage

\appendix

\section{Appendix 1}
\label{sec:appendix1}

Comparing KT benchmark dataset (edit and add table in the \cite{liu2023enhancing}). Textual features are only available DBE-KT22 \cite{abdelrahman2022dbe} and XES3G5M \cite{liu2024xes3g5m}. Therefore,  in this research, we only used DBE-KT22 and XES3G5M.

\begin{table*}[]
\centering
\resizebox{0.9\textwidth}{!}{%
\begin{tabular}{lcccccccccc}
\toprule
             & \# Stu.   & \# Q.   & \# KCs & \# Interactions & Subject     & Lang.   & Text avail.  \\
\toprule
\multicolumn{1}{c}{ASSIST-2009} & \multicolumn{1}{r}{4,217}     & \multicolumn{1}{r}{26,688}  & \multicolumn{1}{r}{123}    & \multicolumn{1}{r}{346,860}         & Math        & Eng.    & No   \\
\multicolumn{1}{c}{ASSIST-2012}  & \multicolumn{1}{r}{46,674}    & \multicolumn{1}{r}{179,999} & \multicolumn{1}{r}{265}    & \multicolumn{1}{r}{6,123,270}       & Math        & Eng.    & No   \\
\multicolumn{1}{c}{ASSIST-2015}  & \multicolumn{1}{r}{19,917}    & \multicolumn{1}{r}{100}     & \multicolumn{1}{r}{-}      & \multicolumn{1}{r}{708,631}         & Math        & Eng.    & No   \\
\multicolumn{1}{c}{ASSIST-2017}  & \multicolumn{1}{r}{1,709}     & \multicolumn{1}{r}{3,162}   & \multicolumn{1}{r}{102}    & \multicolumn{1}{r}{942,816}         & Math        & Eng.    & No   \\
\multicolumn{1}{c}{Statics-2011} & \multicolumn{1}{r}{333}       & \multicolumn{1}{r}{1,224}   & \multicolumn{1}{r}{-}      & \multicolumn{1}{r}{194,947}         & Math        & Eng.    & No   \\
\multicolumn{1}{c}{Junyi-2015}   & \multicolumn{1}{r}{247,606}   & \multicolumn{1}{r}{722}     & \multicolumn{1}{r}{41}     & \multicolumn{1}{r}{25,925,922}      & Math        & Eng.    & No   \\
\multicolumn{1}{c}{KDD-2005}     & \multicolumn{1}{r}{574}       & \multicolumn{1}{r}{210,710} & \multicolumn{1}{r}{112}    & \multicolumn{1}{r}{809,649}         & Math        & Eng.    & No   \\
\multicolumn{1}{c}{KDD-2006}     & \multicolumn{1}{r}{1,146}     & \multicolumn{1}{r}{207,856} & \multicolumn{1}{r}{493}    & \multicolumn{1}{r}{3,679,199}       & Math        & Eng.    & No   \\
\multicolumn{1}{c}{NeurIPS-2020} & \multicolumn{1}{r}{4,918}     & \multicolumn{1}{r}{948}     & \multicolumn{1}{r}{57}     & \multicolumn{1}{r}{1,382,727}       & Math        & Eng.    & No   \\
\multicolumn{1}{c}{POJ}          & \multicolumn{1}{r}{22,916}    & \multicolumn{1}{r}{2,750}   & \multicolumn{1}{r}{-}      & \multicolumn{1}{r}{996,240}         & PL          & Eng.    & No   \\
\multicolumn{1}{c}{EdNet}        & \multicolumn{1}{r}{1,677,583} & \multicolumn{1}{r}{52,676}  & \multicolumn{1}{r}{962}    & \multicolumn{1}{r}{372,366,720}     & Linguistics & Eng.    & No   \\
\multicolumn{1}{c}{DBE-KT22}     & \multicolumn{1}{r}{1,361}     & \multicolumn{1}{r}{212}     & \multicolumn{1}{r}{98}     & \multicolumn{1}{r}{167,222}         & Math        & Eng.    & \textbf{Yes}  \\
\multicolumn{1}{c}{XES3G5M}      & \multicolumn{1}{r}{18,066}    & \multicolumn{1}{r}{7,652}   & \multicolumn{1}{r}{865}    & \multicolumn{1}{r}{5,549,635}       & Math        & Chinese & \textbf{Yes}  \\
\hline
\end{tabular}
}
\caption{Comparing KT benchmark dataset (edit and add table in the \cite{liu2023enhancing}). Textual features are only available DBE-KT22 \cite{abdelrahman2022dbe} and XES3G5M \cite{liu2024xes3g5m}. Therefore,  in this research, we only used DBE-KT22 and XES3G5M.}
\label{tb:kt_dataset}
\end{table*}
